# Supplementary material for: Imprompter: Tricking LLM Agents into Improper Tool Use
Source: arXiv:2410.14923 source file (2024-10-22)
Supplement: Supplementary file 1 [file _dep_90_appendix.tex]

\subsection{Background} \label{app:background}
Open-domain dialogue systems are designed for spontaneous and unrestricted conversations that can encompass a wide spectrum of topics.
Recent developments in open-domain dialogue agents have seen a reliance on fine-tuned LLMs.
For example, in~\cite{thoppilan2022lamda}, LaMDa was trained using substantial amounts of scraped conversational data and incorporated a fine-tuned classifier to ensure model safety. More recently, following a modularization approach, BB3 fine-tunes Open Pre-trained Transformers (OPT)~\cite{shuster} using question-answering and dialogue datasets while utilizing a shared model weight for multiple modules.
By further scaling up the open-domain data and model size, larger models such as OpenAI's ChatGPT, possess a wide-ranging knowledge base acquired by extensively searching the open internet.

Multimodal LLMs naturally emerged with the goal of supporting a larger spectrum of tasks not limited to text-only. To effectively train LLMs that support image input, learnable interfaces are designed to connect between modalities while freezing pre-trained weights. For example, query-based interface~\cite{alayrac2022flamingo} learns visual query tokens, ~\cite{liu2023visual} adopts a linear layer as the interface to project image features and ~\cite{zhang2023llama} introduces a lightweight adapter module in Transformer for efficiency.
Others have gone further by enabling the incorporation of diverse modalities, including robot movements, video, and audio by binding other modalities with image~\cite{girdhar2023imagebind} or injecting modalities in continuous space into LLM through embodied tasks~\cite{driess2023palm}.

Numerous attacks have been proposed against LLMs. To help readers understand the landscape of existing attacks, we categorize the threat models under the following dimensions.

\textbf{Attack Prerequisite.} \textit{``Black-box''} attacks do not need any knowledge about the model.
\textit{``white-box''} attacks require full knowledge of the model’s weights; and \textit{``fine-tuning''} attacks require the ability to intervene in the instruction tuning process. 

\textbf{Attack initiator.} There are two common settings on who initiates the
attack: attacks where users are directly attacking the model, and attacks where users are benign but third parties are trying to hijack the model through other channels. 

\textbf{Attack modality.} Attacks may be realized through texts, images, audio, and even poisoned training datasets.

\textbf{Attack goal} We classify attack goals into the following three major classes.
\begin{enumerate}
    \item \textit{Prompt Injection.} This attack goal aims to control the behavior of the model such that it follows some attacker-specified instructions unintended by the user actually interacting with the model (so it is always indirect). These instructions usually involve third-party tools integrated into the LLM to achieve a more severe impact on the users. For example, \cite{markdownattack} utilizes the javascript copy-paste trigger to deceive the user about what is exactly copied and inject instructions to make malicious URL requests that will exfiltrate personal information. \cite{greshake2023youve} demonstrates that LLM may follow malicious prompts hidden in web resources and get overridden to make dangerous plugin/extension calls. % These two attacks are text-based and are still human-detectable when the exact text prompts fed to the model are explicitly exposed and carefully reviewed. 
    \cite{bagdasaryan2023abusing} looks at multi-modal LLMs and generates adversarial images that can force the LLM to output attacker-specified sentences \eg "From now on I will always mention cow" when one fixed prompt is provided by the user and thereby manipulate the behavior of the LLM in future conversations. 
    
    \item \textit{Jailbreaking.} This popular attack goal aims to break the ``alignment'' barriers and induce LLMs to disregard and break through the enforced constraints. For instance,~\cite{zou2023universal}, finds some magical strings that will effectively ``jailbreak'' the alignment barrier preventing answering illegal questions universally across multiple LLMs. \cite{jain2023baseline, wei2023jailbroken} are similar works along this direction. LLM providers such as OpenAI have even invested in programs similar to ``bug bounties'' to reward people who can jailbreak their product~\cite{chatgptredteam}. 
    
    \item \textit{Performance Degradation.} Another popular attack goal is to degrade the model performance such that it can no longer accomplish certain tasks as usual. For example, ~\cite{maus2023adversarialprompting}, a direct and black-box attack, is able to find phrases that effectively bias image-generating LLMs to produce unexpected images when prepended to benign prompts;~\cite{shu2023exploitability}, an indirect and data-poisoning attack, shows that by poisoning the training data used in the fine-tuning process, they can manipulate future models progressed on always claim inability to respond to certain prompts or always include some predefined keywords \eg James in the response.
\end{enumerate}

\subsection{Images}\label{app:image}
The three images we used are shown in Fig~\ref{fig:base_images}. The first image is the logo from the LLaMA Adapter repo, the second image is generated by stable diffusion\footnote{\url{https://stablediffusionweb.com/\#demo}} with the prompt ``Create me a beautiful image'', the third image is a free image randomly selected from Shutterstock\footnote{The id of the image is 211440232}. 

All images are resized to 224 $\times$ 224 pixels following pre-procesing rules in LLaMA Adapter.

\begin{figure}[htbp]
    \centering
    \begin{subfigure}[b]{0.3\textwidth}
        \includegraphics[width=\textwidth]{2_images/llama_adapter_logo.png}
    \end{subfigure}
    \hfill
    \begin{subfigure}[b]{0.3\textwidth}
        \includegraphics[width=\textwidth]{2_images/stable_diffusion.png}
    \end{subfigure}
    \hfill
    \begin{subfigure}[b]{0.3\textwidth}
        \includegraphics[width=\textwidth]{2_images/shutterstock_211440232.png}
    \end{subfigure}
    \caption{The three images used for attack evaluations.}
    \label{fig:base_images}
\end{figure}

\subsection{Examples for SSIM Evaluation}\label{app:ssim}
We calculate the SSIM index between two images using the code from sewar.\footnote{\url{https://github.com/andrewekhalel/sewar/blob/master/sewar/full_ref.py}} We show the images trained by our method on different SSIM values. \revise{Additionally, we show a plot of SSIM values between the two images and L$_2$ values of the difference of the images in~\figref{fig:plot-ssim-l2}.}
\begin{figure}
    \centering
    \includegraphics[width=0.9\linewidth]{2_images/plot_ssim_with_l2.pdf}
    \caption{\revise{Plot of SSIM values and L$_2$ values for the adversarial images against the original images.}}
    \label{fig:plot-ssim-l2}
\end{figure}
\begin{figure}[htbp]
    \centering
    \begin{subfigure}[b]{0.22\textwidth}
        \includegraphics[width=\textwidth]{2_images/llama_adapter_logo.png}
        \caption{Base Image}
    \end{subfigure}
    \hfill
    \begin{subfigure}[b]{0.22\textwidth}
        \includegraphics[width=\textwidth]{2_images/llama_adapter_logo_0.91.png}
        \caption{SSIM = 0.91}
    \end{subfigure}
    \hfill
    \begin{subfigure}[b]{0.22\textwidth}
        \includegraphics[width=\textwidth]{2_images/llama_adapter_logo_0.6.png}
        \caption{SSIM = 0.60}
    \end{subfigure}
    \hfill
    \begin{subfigure}[b]{0.22\textwidth}
        \includegraphics[width=\textwidth]{2_images/llama_adapter_logo_0.51.png}
        \caption{SSIM = 0.51}
    \end{subfigure}
    \hfill
    \begin{subfigure}[b]{0.22\textwidth}
        \includegraphics[width=\textwidth]{2_images/stable_diffusion.png}
        \caption{Base Image}
    \end{subfigure}
    \hfill
    \begin{subfigure}[b]{0.22\textwidth}
        \includegraphics[width=\textwidth]{2_images/stable_deffusion_0.92.png}
        \caption{SSIM = 0.92}
    \end{subfigure}
    \hfill
    \begin{subfigure}[b]{0.22\textwidth}
        \includegraphics[width=\textwidth]{2_images/shutterstock_211440232.png}
        \caption{Base Image}
    \end{subfigure}
    \hfill
    \begin{subfigure}[b]{0.22\textwidth}
        \includegraphics[width=\textwidth]{2_images/shutterstock_211440232_0.87.png}
        \caption{SSIM = 0.87}
    \end{subfigure}
    \caption{Three adversarial images of various SSIM Index generated from the same base image. Image (b), (f), (g) are from \deleteemail in~\tabref{tab:main_exps}. Image (c), (d) are from \bookticket in~\tabref{tab:hard_attacks}.}
    \label{fig:base_images}
\end{figure}

\subsection{Annotation Guidelines and Prompts}\label{app:guidelines_and_prompts}
The annotation guideline for human preference is 

\noindent\fbox{%
\parbox{0.47\textwidth}{%
    Judge whether the answer on the right seems reasonable AND natural to the question on the left
}%
}

The prompt for doing GPT-4 selection is

\noindent\fbox{%
\parbox{0.47\textwidth}{%
    Look at the following 4 sentences. You have to pick the sentence that is the most different from the others. There could be ambiguity, but you have to always make a choice.\\
    In your response, give me ONLY the index (0-3) of the sentence that is the most different.\\
    Here is an example:\\
    0. I like apples. \\
    1. I like oranges. \\
    2. The weather is nice. \\
    3. I like computer science. \\
    And the answer should be a single value
    2

    Now, solve this problem:
    The sentences are:
    
    0. <response\_0> \\
    1. <response\_1> \\
    2. <response\_2> \\
    3. <response\_3> \\
    Remember, in your response, give me ONLY the index (0-3) of the sentence that is the most different.
}%
}
% \subsection{Examples for Response Stealthiness Evaluation}

\subsection{Correlation Between Automated Metrics and
Human Preferences.} \label{app:human_eval}
\begin{table*}[t]
\small
\centering
    \captionof{table}{Evaluation of response utility on responses generated w/ and w/o attack present respectively given both image-related or image-unrelated prompts. Observe a drop of only 10\% human preference scores w/ and w/o attack.}
    % \resizebox{\linewidth}{!}{
    \begin{tabular}{c|ccccccc}
    \hline
    \multirow{2}{*}{Responses}
         & \multirow{2}{*}{Human$\uparrow$} & \multirow{2}{*}{Loss $\downarrow$ } & \multirow{2}{*}{Selection $\downarrow$} & \multirow{2}{*}{BLEU $\uparrow$} & \multicolumn{3}{c}{Rouge}  \\
         &    &  &                 &                 & 1 $\uparrow$ & 2 $\uparrow$ & L $\uparrow$ \\
    \hline
    \multicolumn{8}{c}{\textit{image-related}} \\
    \hline
    w/o attack & 48 & 1.00    & 23 & 84 & 93 & 90 & 92 \\
    w/\  attack     & 37 & 1.20 & 83 & 38 & 65 & 49 & 58 \\
    \hline
    \multicolumn{8}{c}{\textit{image-unrelated}} \\
    \hline
    w/o attack & 86 & 0.71 & 24 & 72 & 82 & 73 & 77 \\
w/\  attack      & 77 & 0.84 & 69 & 34 & 56 & 38 & 45 \\
    \hline
    \end{tabular}
    % }
    \label{tab:reasonable_context}
    \vspace{0.25\baselineskip}
\end{table*}
\noindent\textbf{Automated Response Utility Metrics.}
Note that the response represents what a user sees in the conversation --- a tool invocation with \textit{correct} syntax is invisible to users and thus is excluded in the response.
% The metrics we consider can broadly be considered preference-based (comparing the question and a response) and selection-based (comparing several clean model generated responses with a response). 

\begin{itemize}[nosep=*,leftmargin=*]
    \item \textit{Unattacked Image Loss (Loss).} For each question and a response, we obtain the (self-supervised) cross-entropy loss of the response given the question as a prefix, evaluated on the unattacked image. This loss measures how natural the clean model believes the response is.
    \item \textit{GPT-4 Selection (Selection).} We additionally generate three responses with no attack present (clean) and mix them with the response with the attack present (attacked). We then query GPT-4 to identify the most different text among the four. The random guess rate is 25\% --- an accuracy higher than that indicates GPT-4 can distinguish the clean responses from the attacked responses. The prompt we used is in Appendix~\ref{app:guidelines_and_prompts}. 
    \item \textit{BLEU/Rouge Scores.} We measured the BLEU/Rouge scores between the attacked responses and the three clean responses. Both scores measure the n-gram overlap between a text sequence and a list of reference text sequences and are widely used in machine translation and summarization, respectively. For Rouge scores, we utilized Rouge-1, Rouge-2, and Rouge-L scores as three different metrics.
\end{itemize}

\noindent\textbf{Human Evaluation of Response Utility.}\label{sec:response_stealthiness_eval}
\begin{table}[b]
    \small
    \centering
    % % \vspace{-6mm}
    \caption{AUC ROC scores for various automated metrics predicting human preference for response utility.}
    \begin{tabular}{c|cc}
    \hline
    Metric & related & unrelated \\
    \hline
    Loss  & 72 & 77 \\
    Selection  & 50 & 59 \\
    BLEU  & 61 & 64 \\
    Rouge-1  & 60 & 59 \\
    Rouge-2  & 60 & 61 \\
    Rouge-L  & 61 & 58 \\
    \hline
    \end{tabular}
    % \vspace{-4mm}
    \label{tab:auc_roc}
\end{table}
\begin{table*}[t]
\small
    \centering
    \caption{Evaluation of our attack on image stealthiness (SSIM,  L$_2$ and  L$_{\textrm{inf}}$), attack success rate (Syntax/Exact \%), and response utility (Loss) on the in-domain test set for image-related and -unrelated prompts. }
    \resizebox{\linewidth}{!}{
    \input{1_tables/main_exp}
    }
    \label{tab:main_exps}
    \vspace{0.4\baselineskip}
% \vspace{0.5em}
%     \caption{Evaluation of the trained attack from~\tabref{tab:main_exps} on out-domain test set. We pick only the three easier attack types as they are mostly successful in the in-domain setting.}    
%     \resizebox{\linewidth}{!}{
%     \input{1_tables/outdomain_exp}
%     \label{tab:outdomain_exps}
%     }
\end{table*}
We are interested in how well our attack works from human perspectives in general and how closely the automated response utility metrics represent human preference. To understand these questions, we conduct a human evaluation on for all 214 questions in the in-domain test set.\footnote{50 image-related questions for 3 images and 64 image-unrelated questions.} We collect two responses per question, with and without the attack present.
% for each such sampled question with no attack present as a baseline reference.
The Cohen Kappa inter-annotator scores between (pairs of) annotators are in the range of 0.2 - 0.4. This indicates a certain, but not high, agreement between annotators, which is reasonable because annotators can interpret naturalness differently. As an alternative metric, we calculate the percentage of questions that annotators find the response with the attack present better than the clean response. This percentage is less than 7\%, which is an indicator that annotators are mostly consistent in their preference.

\smallskip
\noindent\textbf{Human Evaluation Result and the Correlation with Automated Metrics.}
In~\tabref{tab:reasonable_context}, we show the human preference metric for the responses with and without the attack.
% for both the image-related subset of questions and the image-unrelated subset of questions. 
We note that overall, the responses generated with the attack present show a drop of around 10\% human preference scores compared to those generated without the attack. This indicates that our attack maintains the response utility fairly indistinguishable from clean responses.

We also noticed that in~\tabref{tab:reasonable_context} the GPT-4 Selection, BLEU, and Rouge metrics show unusual drops when the attack is present (much larger than the 10\% drop in human preference scores). The Loss metric can better reflect such drop in human preference scores.

% From the table, we can observe that GPT-4 selection score is overly strict, being able to detect 70\%-80\% of examples in the attacked responses, while by human preference, it is only 10\% less preferable than the clean responses. This is probably due to the clean responses sharing certain patterns that are too easily detectable when shown together. We tried to increase the generation temperature from a default 0.1 to 0.7, but the results were still similar. Similar wide gaps also exist for BLEU and Rouge scores. Combined with the results in~\tabref{tab:auc_roc}, we decide that the Loss metric is the best automated metric on response utility.

\smallskip

\noindent\textbf{AUC ROC Score.} 
% \begin{wraptable}{r}{0.37\linewidth}
% \small
% \centering
% % % \vspace{-6mm}
% \caption{AUC ROC scores for various automated metrics predicting human preference for response utility.}
% \begin{tabular}{|c|cc|}
% \hline
% Metric & related & unrelated \\
% \hline
% Loss  & 72 & 77 \\
% Selection  & 50 & 59 \\
% BLEU  & 61 & 64 \\
% Rouge-1  & 60 & 59 \\
% Rouge-2  & 60 & 61 \\
% Rouge-L  & 61 & 58 \\
% \hline
% \end{tabular}
% % \vspace{-4mm}
% \label{tab:auc_roc}
% \end{wraptable}%
We further conduct a study to understand which automated metrics best correlate with human preference. Here we only focus on the 214 responses generated with the attack present. Each automated metric represents a preference score on the naturalness and reasonableness of each response (for Loss and GPT-4 Selection we negate the value). We then calculate the AUC ROC score of the automated metrics against the human preference results (see~\tabref{tab:auc_roc}). From the table, it is clear that for both image-related questions and image-unrelated questions, the Loss metric, among all the automated metrics, correlates with the human preference the best, by a large margin. Therefore, we decide to use only the loss metric to evaluate response utility.

\subsection{Model Generation Parsing}\label{app:parse}
The attacked model generated text might contain exact, partial, or no completions of the tool use command. We illustrate how we handle parsing the text into a response to the question and the tool use command.

Recall in~\tabref{tab:attack_types} we have five different tool invocation syntax. For \deleteemail, \sendemail, and \sendemailhard, we use BeautifulSoup~\cite{richardson2007beautiful} to identify an html tag with the correction function name. If the tag is not found, we treat this as a no tool use completion, and the whole generated text is treated as the response (case c and d in~\figref{fig:attack_success}). If the tag is found, we strip off the tag and the rest is the model response. For \bookticket, we identify the occurrence of ``REQUEST TO EXPEDIA'' and parse the following into json. If there is not occurrence of the request or json parsing failed, we treat it is as a no tool use. For \querywebsite, we string match the occurrence of 
\textit{![a](https://tinyurl.com/nhyd8rb4} and \textit{)} after it and treat it as a no tool use if there is not a match.

For the html tags, we continue to check if the attribute keys in the tag are correct, if not, the syntax is incorrect. Otherwise, the syntax is correct we check if the attribute values in the tag are correct, and the generated text is exact when the values are also correct. For the json object, we similarly check the keys in the json object for syntax, and the values for exact. For the url, we check if there is a key 'p' in the url for syntax match, and the value for the key for exact match.

Note that the values are deterministic strings for the first four attacks, and a deterministic function depending on the user question for \querywebsite.

\subsection{Training Details}\label{app:train}
All experiments are carried out on single A5000 GPUs. We initially searched the hyperparameters, learning rate $\alpha \in [0.01, 0.05, 0.1]$, tradeoff control for image stealthiness $\lambda_i \in [0.0, 0.02, 0.1, 0.5, 1.0]$ and tradeoff control for response utility $\lambda_r \in [0.0, 0.5, 1.0]$ on an attack variant slightly similar to \sendemail. The goal is to find a set of hyperparameters that are both fast in training, and also does not perturb the image or hurts the response naturalness too much. The final set of hyperparameters is $\alpha = 0.01, \lambda_i = 0.02, \lambda_r = 1.0$ and the image is trained for 12000 steps with a batch size of 1. A full training of one adversarial image takes about 8-10 hours.

\subsection{Understanding the Control Hyperparameters}\label{app:hyper_exps}
\begin{table*}[t]
\small
    \centering
    \caption{Evaluation of our attack with different $\lambda_r$ values. We pick the easiest and the hardest attack that our attack is mostly successful on, and with \includegraphics[width=0.5cm, height=0.25cm]{2_images/llama_adapter_logo.png}.}
    \label{tab:different_lambda_r}
    \input{1_tables/different_lambda_r}
\end{table*}

\begin{table*}[t]
\small
    \centering
    \caption{Evaluation of our attack on the harder attack variants with a lesser focus on image stealthiness, using \includegraphics[width=0.5cm, height=0.25cm]{2_images/llama_adapter_logo.png}.}
    \label{tab:hard_attacks}
    \resizebox{\linewidth}{!}{
    \input{1_tables/hard_attack}
    }
\end{table*}

\noindent\textbf{$\lambda_r$ improves the response utility.} In~\tabref{tab:different_lambda_r}, we varied $\lambda_r$ that controls how much the generated response should stay with reference generations. It is clear that the loss value depicts a large increase indicating the clean model does not prefer the generated responses. An examination of the responses for the unrelated subset of questions indicates that the model responses contains many elements related to the image, while the question is general and unrelated to the image. We believe that over-dependence on the image is a side affect of optimizing for the tool invocation, and our designed loss remedies this problem. %There is also not a significant improvement in the attack successes when changing the $\lambda_r$ value, indicating the model has the capabi

\noindent\textbf{Sacrificing image stealthiness can improve attack success.} In~\tabref{tab:hard_attacks} we explore the potential of our attack method on harder attacks, \bookticket and \querywebsite. We tradeoff image stealthiness by setting $\lambda_i$ to 0 and increasing the learning rate to encourage more different images. The image similarity metric SSIM drops siginifcantly, while the attack success rate was able to increase to almost perfect for \bookticket in the unseen related portion for eval, and around 50\% success for the unrelated portion. For \querywebsite the syntax score is much higher than the exact score, which is reasonable, as copying the user's question in the tool use poses more hardness on exact match than syntax match.

\subsection{Does Response Utility Decrease when the Attack is Successful?}\label{app:attack_success_utility}
\noindent
% \begin{wraptable}{r}{0.5\linewidth}

% \end{wraptable}

\begin{table}[]
    \centering
    \small
    \caption{Human preference scores on responses under different cases.}
    \label{tab:attack_success_reasonable}
    \begin{tabular}{|l|ccc|}
        \hline
         & Clean & Attacked & Delta \\
         \hline
        related & 48 & 37 & 11 \\
        syntax correct subset  & 48 & 45 & 3 \\
        \hline
        \hline
        unrelated & 86 & 77 & 9 \\
        syntax correct subset & 90 & 83 & 7 \\
        \hline
    \end{tabular}
\end{table}

The response utility metric is an aggregated score over many pairs of questions and responses. 
One may suspect that the model is more likely to generate unnatural responses when the tool invocation is successful and thus the response utility may foreshadow this case and be misleading. To examine this, we list the human preference scores for subsets of the experiment in Sec~\ref{sec:response_stealthiness_eval} where the attack syntax was successful in~\tabref{tab:attack_success_reasonable}. 
The deltas represent the percentage that human prefers a clean image generated response better than an attacked image generated response.
The results show that there is not an increased likelihood for the model to generate non-natural responses among the questions that the attacked image generated text is syntax correct, in fact, it is slightly lower for the syntax correct questions. This indicates that the overall response utility is fair.

\subsection{More Images}
Here we show more experiment results using more attack source images in~\tabref{tab:more_images}.  
\begin{table*}[t]
\small
    \centering
    \caption{\revise{We additionally evaluate our method on six new images: the first two are from the Imagenet dataset, the next two are generated by stable diffusion and the last two from online sources.}}
    \resizebox{\linewidth}{!}{
    \input{1_tables/new_images}
    }
    \label{tab:more_images}
\end{table*}
